# Supplementary material for: Self-Contained Kinematic Calibration of a Novel Whole-Body Artificial Skin for Human-Robot Collaboration
Source: arXiv:2110.14516 source file (2021-10-27)
Supplement: Supplementary file 1 [file appendix.tex]

\section*{APPENDIX}

Appendixes should appear before the acknowledgment.
